# Supplementary material for: Explainable 3D Convolutional Neural Networks by Learning Temporal Transformations
Source: arXiv:2006.15983 source file (2020-06-29)
Supplement: Supplementary file 1 [file supplementary.tex]

ResNet18 \cite{he2016deep}
GoogLeNet \cite{szegedy2015going}
Jester dataset \cite{materzynska2019jester}
UCF101 dataset \cite{soomro2012ucf101}

- choose deconv, activation-maximization, gradient-based, first layer filters, SRXY plots
- for both datasets, show results with non-pretrained resnet and googlenet
- introduce idea of pre-training
- show results with pre-trained resnet and googlenet

In the following experiments we compare our method to existing alternatives, specifically, (i) visualizing first layer filters, (ii) deconvolution \cite{zeiler14} and (iii) activation maximization \cite{erhan2009visualizing}.

We train our model on the Jester dataset \cite{materzynska2019jester}. A gesture recognition dataset with 27 classes.

We modify a ResNet18 that has been pre-trained on ImageNet by replacing 2DConv with 3TConv and copying the pre-trained ImageNet weights to the weights of 3TConv. The transformation parameters are set to identity. We finetune using ADAM with a learning rate of $5e-5$ using early stopping. To manage class imbalance we implement a weighted loss. For further pre-processing of the Jester dataset see details in Appendix \ref{app:jester}. The fine-tuned model reaches an accuracy of $xx\%$ on the training split and $xx\%$ on the validation split. 

As a comparison to show that pre-training really works we can compare with a modified ResNet18 where the 2DConv has been replaced by 3TConv, but where no pre-training has taken place. The model trains directly on Jester without pre-training on ImageNet. The model is trained using ADAM and learning rate of $5e-5$ using early stopping. The trained model reaches an accuracy of $xx\%$ on the training split and $xx\%$ on the validation split.

% 3DConv: 
% ji20123d: 3D CNN
% varol2017long: LTC-CNN
% tran2015learning: C3D
% carreira2017quo: I3D
